# Supplementary material for: MOOMIN: Deep Molecular Omics Network for Anti-Cancer Drug Combination Therapy
Source: arXiv:2110.15087 source file (2022-08-08)
Supplement: Supplementary file 1 [file appendix.tex]

\appendix

\section{Multi-scale node representations} These techniques encode location and node attribute information coming from increasing orders of proximity in the graph with separate blocks of representations for each node. We summarized how these techniques differ from each other in Table \ref{tab:related_multi} based on these desirable characteristics:

\begin{itemize}
    \item \textbf{Supervised:} Node level embeddings can be trained to be optimal with respect to a downstream machine learning task.
    \item \textbf{Implicit:} The higher-order proximity matrix (e.g. random walk based pointwise mutual information) of nodes is not calculated explicitly by the model.
    \item \textbf{Attributed:} Vertex representations are learned by the distribution of generic attributes in the neighbourhoods not just pairwise node proximity.
    \item \textbf{Multimodal:} The attributes of vertices which are described by various data modalities (e.g. image, sound, text) can be incorporated by the model.
    \item \textbf{Inductive:} The representations of new nodes can be inferred without updating the model weights or learning a representation for the new node.
\end{itemize}

Based on our understanding MOOMIN is the first multi-scale node representation learning algorithm which incorporates multimodal data.

\begin{table}[h!]
\centering
\caption{A desiderata based comparison of MOOMIN and existing unsupervised and supervised multi-scale node representation learning algorithms.}\label{tab:related_multi}
\setlength{\tabcolsep}{2pt}

{\footnotesize
\begin{tabular}{ccccccc}
\toprule
\textbf{Method}&   \textbf{Implicit} & \textbf{Supervised} &\textbf{Attributed} & \textbf{Inductive} & \textbf{Multimodal}  \\
\hline 
 LINE \cite{tang2015line}& $\bullet$ &   &   &   &   \\
 GraRep \cite{cao2015grarep}&   &   &   &   &   \\
 Walklets \cite{perozzi2017don}&$\bullet$  &   &   &   &   \\
 MUSAE \cite{rozemberczki2019multi}& $\bullet$ &   & $\bullet$ &  &     \\
 \hline 
 FEATHER \cite{rozemberczki2020characteristic}& $\bullet$  & $\bullet$  & $\bullet$  &$\bullet$  &      \\
 MixHop \cite{abu2019mixhop}& $\bullet$  & $\bullet$  & $\bullet$  &$\bullet$  &      \\
SkipGNN \cite{huang2020skipgnn}&   & $\bullet$  & $\bullet$  &$\bullet$  &      \\
 HWGNN \cite{liu2019higher}& $\bullet$  & $\bullet$  & $\bullet$  &$\bullet$  &      \\
 SIGN \cite{rossi2020sign}& $\bullet$  &  $\bullet$ & $\bullet$  & $\bullet$ &       \\
 MOOMIN (ours) &$\bullet$  &$\bullet$  & $\bullet$ &$\bullet$ &$\bullet$     \\
\bottomrule
\end{tabular}
}
\end{table}
\vspace{-5mm}
